# Supplementary material for: Effectively Unbiased FID and Inception Score and where to find them
Source: arXiv:1911.07023 source file (2020-06-15)
Supplement: Supplementary file 1 [file supplementary.pdf]

## Appendix

Pseudo-code for calculating  $\overline{\text{FID}}_\infty$ . Evaluating  $\overline{\text{IS}}_\infty$  is exactly the same except swapping the FID calculation function for IS calculation function.

---

**Algorithm 1** Evaluating  $\overline{\text{FID}}_\infty$  for a Generator

---

```
1:  $G$ : Generator
2:  $I$ : Inception Network
3:  $n$ : Number of images we want to generate
4:  $t$ : Number of FIDs we compute for extrapolation
5:  $m_t$ : Precomputed groundtruth activations mean
6:  $c_t$ : Precomputed groundtruth activations covariance
7:
8: procedure EVALUATE( $G, I, n, t, m_t, c_t$ )
9:    $\text{FID} = \{\}$ 
10:   $z \leftarrow \text{SOBOLSAMPLER}(n)$ 
11:   $\text{activations} \leftarrow I(G(z))$ 
12:
13:   $\triangleright$  5000 is the min no. of images we evaluate with
14:   $\text{batchSizes} = \text{Linspace}(5000, n, t)$ 
15:  for batchSize in batchSizes do
16:    SHUFFLE(activations)
17:     $\text{activations}_i \leftarrow \text{activations}[:\text{batchSize}]$ 
18:     $\text{FID.insert}(\text{CALCULATEFID}(\text{activations}_i,$ 
19:       $m_t, c_t))$ 
20:  end for
21:   $\text{reg} \leftarrow \text{LINEARREGRESSION}(1/\text{batchSizes}, \text{FID})$ 
22:   $\overline{\text{FID}}_\infty \leftarrow \text{reg.predict}(0)$ 
23:  return  $\overline{\text{FID}}_\infty$ 
end procedure
```

---

```

1 from botorch.sampling.qmc import NormalQMCEngine
2
3 class randn_sampler():
4     """
5     Generates  $z \sim N(0,1)$  using random sampling or scrambled Sobol sequences.
6     Args:
7         ndim: (int)
8             The dimension of z.
9         use_sobol: (bool)
10            If True, sample z from scrambled Sobol sequence. Else, sample
11            from standard normal distribution.
12            Default: False
13         use_inv: (bool)
14            If True, use inverse CDF to transform z from  $U[0,1]$  to  $N(0,1)$ .
15            Else, use Box-Muller transformation.
16            Default: True
17         cache: (bool)
18            If True, we cache some amount of Sobol points and reorder them.
19            This is mainly used for training GANs when we use two separate
20            Sobol generators which helps stabilize the training.
21            Default: False
22
23     Examples::
24
25         >>> sampler = randn_sampler(128, True)
26         >>> z = sampler.draw(10) # Generates [10, 128] vector
27     """
28
29     def __init__(self, ndim, use_sobol=False, use_inv=True, cache=False):
30         self.ndim = ndim
31         self.cache = cache
32         if use_sobol:
33             self.sampler = NormalQMCEngine(d=ndim, inv_transform=use_inv)
34             self.cached_points = torch.tensor([])
35         else:
36             self.sampler = None
37
38     def draw(self, batch_size):
39         if self.sampler is None:
40             return torch.randn([batch_size, self.ndim])
41         else:
42             if self.cache:
43                 if len(self.cached_points) < batch_size:
44                     # sample from sampler and reorder the points
45                     self.cached_points = self.sampler.draw(int(1e6) [torch.randperm(int(1e6))])
46
47                     # Sample without replacement from cached points
48                     samples = self.cached_points[:batch_size]
49                     self.cached_points = self.cached_points[batch_size:]
50                     return samples
51             else:
52                 return self.sampler.draw(batch_size)

```

Listing 1: PyTorch code for generating Sobol points
